# Supplementary material for: Coordinated Online Learning With Applications to Learning User Preferences
Source: arXiv:1702.02849 source file (2017-02-09)
Supplement: Supplementary file 1 [file appendix_adagrad.tex]

%!TEX root = ../aistats-co-ol-hemimetrics.tex

%%%%%%%%%%%%%%%%%%%%%%%%%%%%%%%%%%%%%%%%%%%%%%%%%%%%%%%%%
%%%%%%%%%%%%%%%%%%%%%%%%%%%%%%%%%%%%%%%%%%%%%%%%%%%%%%%%%
%\section{Proof of Theorem~\ref{thm.regretbounds}}\label{appendix1_theorem1-proof}

\begin{proofsection}{Proof of corollary \ref{corollary:adagrad}}
\subsubsection*{Preparation}
We define $\w^t$ and $\gradient^t$ as the concatenated problem specific vectors
$$
\w^t=\begin{bmatrix}
 \w^t_1  \\
\vdots \\
 \w^t_\problems  \\
\end{bmatrix}
\qquad
\gradient^t=\begin{bmatrix}
\gradient^t_1 \\
\vdots \\
\gradient^t_\problems
\end{bmatrix}
.
$$

Note that $\w^t$ $\gradient^t$ are $0$ in all positions that do not correspond to problem $\z$ at time $t$.

Further, we define the outer product gradient matrix as 
$$\pmb{G}^{t} = \sum^t_{s=1} \gradient^s \otimes \gradient^s $$

and 
$$\regularizer^t(\w) = \frac{1}{2} \w \cdot (\pmb{G}^{t})^{1 / 2} \w .$$

\subsubsection*{\AdaGrad algorithm}
Algorithm \ref{alg:AdaGrad} is a simplified version of the \AdaGrad algorithm with the above notation, setting the algorithmic parameter $\varphi=0$.

%\begin{algorithm}[H]
%  \caption{\AdaGrad} \label{alg:AdaGrad}
%  \begin{algorithmic}[1]
%    \Input{$\eta \geq 0$}
%	\Initialize{$\w^1_\z \in \solutionspace_\z$ for all $\z$}
%	\Statex
%		\For{$t \gets 1 \textrm{ to } T$}
%		\State predict $\prediction^t$
%		\State calculate $\gradient^t$
%		\State update $\w^{t+1} = \argmin_{\w \in \solutionspace} \eta \gradient^t \cdot \w + \divergence_{\regularizer^t}(\w, \w^t)$
%	\EndFor
%  \end{algorithmic}
%\end{algorithm}

%%%%%%%%%%%%%%%%%%%%%%%%%%%%%%%%%%%%%%%%%%%%%%%%%%%%%%%%%%

\begin{algorithm}[H]
\nl 	{\bfseries Input:} $\eta \geq 0$\\
\nl 	{\bfseries Initialize:} {$\w^1_\z \in \solutionspace_\z$ for all $\z$}
\nl	\For{$t = 1, 2, \ldots, T$}{ 
\nl		predict $\prediction^t$ \\
\nl		calculate $\gradient^t$ \\
\nl		update $\w^{t+1} = \argmin_{\w \in \solutionspace} \eta \gradient^t \cdot \w + \divergence_{\regularizer^t}(\w, \w^t)$ \\
	}
	\caption{\AdaGrad}  
	\label{alg:AdaGrad}
\end{algorithm}	
%%%%%%%%%%%%%%%%%%%%%%%%%%%%%%%%%%%%%%%%%%%%%%%%%%%%%%%%%%

We next proof that the equivalence of the update step of \AdaGrad and \COCP.

\subsubsection*{Update equivalence}
Using $\gradient^t_\z \in \{-1, 1\}$ and representing the number of times problem $\z$ was observed until time $t$ as  $\counter^t_\z$,

$$\pmb{G}^{t} = \sum^t_{s=1} \gradient^s \otimes \gradient^s = \sum^t_{s=1} \begin{bmatrix}
(\gradient^t_1)^2 & & 0  \\
& \ddots & \\
0 & & (\gradient^t_\problems)^2
\end{bmatrix}
=
\begin{bmatrix}
\counter^t_1 & & 0  \\
& \ddots & \\
0 & & \counter^t_\problems
\end{bmatrix} 
=
(\Q^t)^2
 $$
and
$$ (\pmb{G}^{t})^{1 / 2} = \Q^t .$$

Thus, we can rewrite 
$$\regularizer^t(\w) = \frac{1}{2} \w \cdot \Q^t \w .$$

Using Lemma \ref{lemma:update2}, we get that the update procedure
$$ \w^{t+1} = \argmin_{\w \in \solutionspace} \eta \gradient^t \cdot \w + \divergence_{\regularizer^t}(\w, \w^t) $$

is equivalent to setting
$$ \wtilde^{t+1} = \w^t - \eta^t_\z \gradient^t $$

and 
$$\w^{t+1} = \argmin_{\w \in \solutionspace} (\w - \wtilde) \cdot \Q^t (\w - \wtilde)$$
\end{proofsection}
