# Supplementary material for: Coordinated Online Learning With Applications to Learning User Preferences
Source: arXiv:1702.02849 source file (2017-02-09)
Supplement: Supplementary file 2 [file appendix_projection-algo.tex]

%!TEX root = ../aistats-co-ol-hemimetrics.tex

%%%%%%%%%%%%%%%%%%%%%%%%%%%%%%%%%%%%%%%%%%%%%%%%%%%%%%%%%
%%%%%%%%%%%%%%%%%%%%%%%%%%%%%%%%%%%%%%%%%%%%%%%%%%%%%%%%%
%\section{Proof of Theorem~\ref{thm.regretbounds}}\label{appendix1_theorem1-proof}

\section{Hemimetric Projection}
Our goal is to develop an algorithm to perform a weighted projection onto the set of bounded hemimetrics. That is, if $H \subset \mathbb{R}^\problems$ is the set of bounded hemimetrics, the algorithm needs to solve
$$\dbold^* = \argmin_{\dbold \in H} (\dbold - \dbold')^T \Q^t (\dbold - \dbold'),$$

where $\dbold' \in \mathbb{R}^\problems$.

This problem is closely related to the matrix nearness problem \cite{brickell2008metric}. While for the projection onto the set of hemimetrics no analytic solution is known \citep{brickell2008metric}, several numeric algorithms exist for similar problems.
%%%\footnote{Next to the presented algorithm we also used ideas from \cite{jaggi2013revisiting} to adopt the Frank-Wolfe algorithm to project onto the hemimetric set. We later abandoned this approach due its to disadvantages in runtime.}.
% \citep{higham1988matrix}

\subsection{Floyd-Warshall algorithm}
The Floyd-Warshall algorithm \cite{floyd1962algorithm}, used in graph theory for solving the all-pairs shortest path problem, has been shown to be equivalent to the downward projection onto the hemimetric set \cite{brickell2008metric,singla2016actively}. While the Floyd-Warshall algorithm does not solve the minimization problem above, it provides a quick way to find a solution in the hemimetric set.

%\cite{sra2004triangle}
\subsection{Metric nearness algorithm for $l_2$ norm}
The metric nearness algorithm, proposed by \cite{brickell2008metric}, returns an approximate solution of the $l_2$ projection onto the metric set, which unlike the set of hemimetrics, also enforces symmetry constraints. The idea of the algorithm is to iteratively fix each triangle inequality until the sum of total changes during a single iteration is smaller than a defined convergence parameter. The advantage of the algorithm lies in its (potentially) fast runtime, as shown by \cite{brickell2008metric}.

\subsection{Projection Algorithm}
Our starting point for the hemimetric projection algorithm is the metric nearness algorithm proposed by 
%\cite{sra2004triangle}
\cite{brickell2008metric}. To project onto the hemimetric set, we generalize the metric nearness algorithm to weighted projection and add non-negativity
%\footnote{For metrics, non-negativity is automatically enforced through symmetry.}
 and upper bound constraints. One drawback of the metric nearness algorithm is that it does not provide any guarantees on the returned solution. For any convergence parameter greater than zero, the algorithm neither guarantees that the solution is in the metric set, nor provides a way to upper bound the distance. To be able to better control the behavior of the projection, we adapt the algorithm by applying the Floyd-Warshall algorithm after every iteration to receive a solution in the hemimetric set. This allows us to control the duality gap and set a suitable convergence parameter.
 
Using $\q \in \mathbb{R}^\problems$ to denote the diagonal entries of the weight matrix $\Q$, and $\delta$ to denote the maximum duality gap, we get the following projection algorithm.

\begin{algorithm}[t!]
\nl	{\bfseries Input:} {$\dbold'$, $\q$, $\maxdualitygapnot$} \\
\nl	{\bfseries Initialize:} 
	{
    \begin{itemize}
    		\item $\eij = 0$ $\forall i, j$ \\
    		\item $\qquad$ $\quad$ $\floyd = \text{FloydWarshall}(\dbold', \e)$ \\
    		\item $\qquad$ $\quad$ $\primal = \norm{\floyd - \dbold'}^2_{\q}$ \\
    		\item $\qquad$ $\quad$ $\dual = 0$ \\
    \end{itemize}
    }
\nl	\While{$\primal - \dual > \maxdualitygapnot$}{
\nl		\For{$i \gets 1 \textrm{ to } \types$}{
\nl			\For{$j \gets 1 \textrm{ to } \types$}{
\nl				\For{$k \gets 1 \textrm{ to } \types$}{
\nl					\If{$i \neq j$ and $i \neq k$ and $j \neq k$}{
\nl						$\vzijk \gets \dik + \dkj - \dij$ \\
\nl						$\theta \gets \eij - \eik - \ekj - \vzijk / \left(\qij^{-1} + \qik^{-1}  + \qkj^{-1}\right)$ \\
\nl						\If{$\theta < -\zijk$}{
\nl							$\theta \gets - \zijk$ \\
						}
\nl						$\eij \gets \eij - \qij^{-1} \theta$ \\
\nl						$\eik \gets \eik + \qik^{-1} \theta$ \\
\nl						$\ekj \gets \ekj + \qkj^{-1} \theta$ \\
\nl						$\zijk \gets \zijk + \theta$ \\
					}
				}
			}
		}
\nl		\For{$i \gets 1 \textrm{ to } \types$}{
\nl			\For{$j \gets 1 \textrm{ to } \types$}{
\nl				\If{$i \neq j$}{
\nl					$\theta \gets \qij (\eij - \dij)$ \\
\nl					\If{$\theta < -\xij$}{
\nl						$\theta \gets - \xij$ \\
					}
\nl					$\eij \gets \eij + \qij^{-1} \theta $ \\
\nl					$\xij \gets \xij + \theta$ \\
\nl					$\vxij \gets \dbold'$  \\
\nl					$\theta\gets \qij (\eij + \dij - \upper)$ \\
\nl					\If{$\theta < -\yij$}{
\nl						$\theta \gets - \yij$ \\
					}
\nl					$\eij \gets \eij - \qij^{-1} \theta $ \\
\nl					$\yij \gets \yij + \theta$ \\
\nl					$\vyij \gets \upper - \dbold'$ \\
				}
			}
		}
%
%	\Statex
%	
\nl		$\primal = \norm{\floyd - \dbold'}^2_{\q}$ \\
\nl		$\dual = -\norm{\e}^2_{\q} - 2(\xbold \cdot \vx + \ybold \cdot \vy + \zbold \cdot \vz)$ \\
\nl		$\floyd \gets \text{FloydWarshall}(\dbold', \e)$ \\
	}
\nl	{\bfseries Return:} $\floyd$
	\caption{HemimetricProjection}	
\end{algorithm}

\begin{algorithm}[t!]
\nl	{\bfseries Input:} {$\dbold'$, $\e$} \\
\nl	{\bfseries Initialize:} {$\floyd = \dbold' + \e$} \\
\nl	\For{$k \gets 1 \textrm{ to } \types$}{
\nl		\For{$i \gets 1 \textrm{ to } \types$}{
\nl			\For{$j \gets 1 \textrm{ to } \types$}{
\nl				\If{$i \neq j$ and $i \neq k$ and $j \neq k$}{
\nl					\If{$\fij > \fik + \fkj$}{
\nl						$\fij \gets \fik + \fkj$ \\
					}
				}
			}
		}
	}
\nl	\For{$i \gets 1 \textrm{ to } \types$}{
\nl		\For{$j \gets 1 \textrm{ to } \types$}{
\nl			\If{$i \neq j$}{
\nl				\If{$\fij < 0$}{		
\nl					$\fij \gets 0$ \\
				}
\nl				\If{$\fij > \upper$}{
\nl					$\fij \gets \upper$ \\
				}					
			}
		}
	}
\nl	{\bfseries Return:} $\floyd$
	\caption{FloydWarshall}	
\end{algorithm}
