# Supplementary material for: Coordinated Online Learning With Applications to Learning User Preferences
Source: arXiv:1702.02849 source file (2017-02-09)
Supplement: Supplementary file 3 [file appendix_theorems_ocp.tex]

%!TEX root = ../aistats-co-ol-hemimetrics.tex

%%%%%%%%%%%%%%%%%%%%%%%%%%%%%%%%%%%%%%%%%%%%%%%%%%%%%%%%%
%%%%%%%%%%%%%%%%%%%%%%%%%%%%%%%%%%%%%%%%%%%%%%%%%%%%%%%%%
%\section{Proof of Theorem~\ref{thm.regretbounds}}\label{appendix1_theorem1-proof}

%\section{Theorems}\label{appendix_theorems}
\begin{proofsection}{Proof of Theorem \ref{theorem:OCP} \citep{zinkevich2003online}} \leavevmode
Define for all $t$, $\wtilde^{t+1}_\z = \w^t_\z - \eta^t_\z \gradient^t_\z$ and $\w^{t+1}_\z = \projection{\solutionspace_\z}{\wtilde^{t+1}_\z}$.
\begin{align*}
\wtilde^{t+1}_\z - \wstar_\z &= (\w^t_\z - \wstar_\z) - \eta^t_\z \gradient^t_\z \\
(\wtilde^{t+1}_\z - \wstar_\z)^2 &= (\w^t_\z - \wstar_\z)^2 - 2  \eta^t_\z \gradient^t_\z \cdot (\w^t_\z -\wstar_\z) + (\eta^t_\z)^2 \norm{\gradient^t_\z}^2 .
\end{align*}

By the generalized Pythagorean theorem, for all $\w \in \solutionspace_\z$ and $\wtilde \in \mathbb{R}^d$, we have
\begin{align*}
(\wtilde - \w)^2 &\geq (\wtilde - \projection{\solutionspace_\z}{\wtilde})^2 +  (\projection{\solutionspace_\z}{\wtilde} - \w)^2 \\
&\geq (\projection{\solutionspace_\z}{\wtilde} - \w)^2 .
\end{align*}

Using $\norm{\gradient^t_\z} \leq \norm{\maxgradient_\z}$, we get 
\begin{align*}
(\w^{t+1}_\z - \wstar_\z)^2 &\leq (\w^t_\z - \wstar_\z)^2 - 2 \eta^t_\z \gradient^t_\z \cdot (\w^t_\z -\wstar_\z) + (\eta^t_\z)^2 \norm{\maxgradient_\z}^2 \\
 \gradient^t_\z \cdot (\w^t_\z -\wstar_\z) &\leq \frac{1}{2 \eta^t_\z} ((\w^t_\z -\wstar_\z)^2 - (\w^{t+1}_\z -\wstar_\z)^2) + \frac{\eta^t_\z}{2} \norm{\maxgradient_\z}^2 .
\end{align*}

The regret sums to
\begin{align*}
\regret_{OCP}(\counter) &= \sum^\counter_{t=1} \gradient^t_\z \cdot (\w^t_\z - \wstar_\z) \
\\
& \leq \sum^\counter_{t=1} \left(\frac{1}{2 \eta^t_\z} ((\w^t_\z -\wstar_\z)^2 - (\w^{t+1}_\z -\wstar_\z)^2) + \frac{\eta^t_\z}{2} \norm{\maxgradient_\z}^2 \right) \
\\
& \leq \frac{1}{2 \eta^1_\z} (\w^1_\z - \wstar_\z)^2 - \frac{1}{2 \eta^\counter_\z} (\w^{\counter+1}_\z - \wstar_\z)^2 + \frac{1}{2}  \sum^\counter_{t=2}\left(\frac{1}{\eta^t_\z} - \frac{1}{\eta^{t-1}_\z} \right) (\w^t_\z - \wstar_\z)^2 \\
& \phantom{\leq} +  \frac{\norm{\maxgradient_\z}^2}{2} \sum^\counter_{t=1} \eta^t_\z \
\\
& \leq \norm{\solutionspace_\z}^2 \left(\frac{1}{2 \eta^1_\z} + \sum^\counter_{t=2}\left(\frac{1}{\eta^t_\z} - \frac{1}{\eta^{t-1}_\z} \right) \right) + \frac{\norm{\maxgradient_\z}^2}{2} \sum^\counter_{t=1} \eta^t_\z \
\\
& \leq \norm{\solutionspace_\z}^2 \frac{1}{2 \eta^{\counter}_\z}  + \frac{\norm{\maxgradient_\z}^2}{2} \sum^\counter_{t=1} \eta^t_\z .
\end{align*}

If we define $\eta^t_\z = \frac{1}{\sqrt{t}} \frac{\norm{\solutionspace_\z}}{\norm{\maxgradient_\z}}$, then
\begin{align*}
\sum^\counter_{t=1} \eta^t_\z &= \frac{\norm{\solutionspace_\z}}{\norm{\maxgradient_\z}} \sum^\counter_{t=1}\frac{1}{\sqrt{t}} \\
& \leq \frac{\norm{\solutionspace_\z}}{\norm{\maxgradient_\z}} \left( 1 + \int^\counter_{t=1} \frac{1}{\sqrt{t}} dt \right) \\
& \leq \frac{\norm{\solutionspace_\z}}{\norm{\maxgradient_\z}} \left(1 + \left[2 \sqrt(t) \right]^\counter_1 \right)  \\
& \leq \frac{\norm{\solutionspace_\z}}{\norm{\maxgradient_\z}} \left(2 \sqrt{\counter} - 1 \right) 
\end{align*}

and thus,
\begin{align*}
\regret_{OCP}(\counter) &\leq \frac{\sqrt{\counter}}{2} \norm{\solutionspace_\z} \norm{\maxgradient_\z} + \left(\sqrt{\counter} - \frac{1}{2} \right) \norm{\maxgradient_\z} \norm{\solutionspace_\z} \\
& \leq \frac{3}{2} \sqrt{\counter} \norm{\solutionspace_\z} \norm{\maxgradient_\z} .
\end{align*} 
\end{proofsection}
