# Supplementary material for: Coordinated Online Learning With Applications to Learning User Preferences
Source: arXiv:1702.02849 source file (2017-02-09)
Supplement: Supplementary file 4 [file appendix_userstudy.tex]

%!TEX root = ../aistats-co-ol-hemimetrics.tex

%%%%%%%%%%%%%%%%%%%%%%%%%%%%%%%%%%%%%%%%%%%%%%%%%%%%%%%%%
%%%%%%%%%%%%%%%%%%%%%%%%%%%%%%%%%%%%%%%%%%%%%%%%%%%%%%%%%
%\section{Proof of Theorem~\ref{thm.regretbounds}}\label{appendix1_theorem1-proof}

%%%%%%%%%%%%%%%%%%%%%%%%%%%%%%%%%%%%%%%%%%%%%%%%%%%%%%%%%%%%%%%%%%%%%
%%%%%%%%%%%%%%%%%%%%%%%%%%%%%%%%%%%%%%%%%%%%%%%%%%%%%%%%%%%%%%%%%%%%%
\section{User Study} \label{appendix:userstudy}
Established in 2008, \names{Airbnb} is an online marketplace that allows ordinary home owners to offer their residences as short term rentals to travelers and other guests. According to \names{Airbnb}, over 2 million apartments are listed worldwide and over 60 million guests have been accommodated so far. This enormous success has also sparked significant interest in \names{Airbnb} in the research community \citep{edelman2014digital, fradkin2014search, zervas2015first, zervas2016rise}.

%\note{Past research on Airbnb paragraph}
%
%\cite{zervas2016rise} Estimating the Impact of Airbnb on the Hotel Industry: Our baseline estimate is that a 1\% increase in Airbnb listings in Texas results in
%a 0.05\% decrease in quarterly hotel revenues.
%
%\cite{edelman2014digital}  test for racial discrimination against
%landlords in the online rental marketplace Airbnb.com. Using a new data set combining
%pictures of all New York City landlords on Airbnb with their rental prices and
%information about quality of the rentals, we show that non-black hosts charge
%approximately 12\% more than black hosts for the equivalent rental.
%
%\cite{zervas2015first} Ratings higher on Airbnb than hotels on TripAdvisor

As an online marketplace, \names{Airbnb} fulfills all essential functions of a market \citep{bakos1998emerging}. Hosts and guests match through search and recommender systems and are given the chance to communicate before entering a transaction. \names{Airbnb} supports guests and hosts after they have agree on the terms of a transaction, taking over the payment process and providing formal insurances and guarantees. For example, hosts are provided insurance for damages in their apartment and guests are refunded in case the apartment does not match its description.

Before deciding on an apartment, guests can observe and compare apartment descriptions, features, images. While specific apartment qualities such as cleanliness, comfort or security are difficult to evaluate solely based on that information, they can be readily observed by experience.  Thus, listings on \names{Airbnb} are a typical example of experience goods \citep{nelson1970information}. As such, customer reviews are essential for evaluation and decreasing product uncertainty.

Further, customer reviews on \names{Airbnb} are important to establish trust between guests and hosts. Renting apartments without any information about the identity of the host may raise several concerns in guests related to their safety and privacy. Thus, lacking traditional ways of establishing trust between guests and hosts \citep{resnick2002trust}, guests may resort to customer reviews to evaluate the sincerity of a host \citep{pavlou2004building, sparks2011impact}.

%https://www.tripadvisor.com/TripAdvisorInsights/n2120/24-insights-shape-your-tripadvisor-strategy

Therefore, the high importance of customer reviews on and its large scale and growth make \names{Airbnb} an ideal marketplace for testing our algorithm. For exploring the viability and benefit of implementing our algorithm, we are interested whether guests in general are willing to accept offers for infrequently reviewed apartments, given sufficient monetary incentive and whether the utility of gaining a review for an infrequently reviewed apartment exceeds the required monetary incentive. Further, if guests are willing to accept discounts that do not exceed the utility of the marketplace, we are interested whether our algorithm can also learn the required incentives over time.

%%%%%%%%%%%%%%%%%%%%%%%%%%%%%%%%%%%%%%%%%%%%%%%%%%%%%%%%%%%%%%%%%%%%%
%%%%%%%%%%%%%%%%%%%%%%%%%%%%%%%%%%%%%%%%%%%%%%%%%%%%%%%%%%%%%%%%%%%%%
\subsection{Utility on Airbnb}
Extending the previous notation, we introduce the utility $\utility_\z$, which summarizes the total gains if a user switches from an apartment of type $\typei$ to an apartment of type $\typej$, corresponding to problem type $\z$. Since we do not have access to the utility function of \names{Airbnb}, we instead resort to the referral program offered on their marketplace. Next to the compensating users for inviting new guests, \names{Airbnb} also provides incentives for referring new hosts. This way, users who invite home owners to list their apartment receive a 75 USD credit once the newly listed apartment has been booked for the first time. Thus, the utility of acquiring a new apartment for \names{Airbnb} is at least that amount.

Further, analyzing the distribution of reviews on \names{Airbnb} (see Table \ref{table:airbnb}), we note that a large fraction of apartments are essentially neglected by potential guests, as long as no reviews are available. Thus, given the high importance of customer reviews for apartments, we argue that from the perspective of \names{Airbnb}, acquiring a new apartment listing is similar to acquiring a review on an infrequently reviewed apartment and that the utility for \names{Airbnb} is in a similar range. 

%While the total utility of a user switching from an apartment of type $\typei$ to an apartment of type $\typej$ cannot be accurately determined, we can estimate the utility for the specific case of a user switching from a frequently reviewed apartment to an infrequently reviewed apartment for the marketplace itself.  Since for many of these apartments, the only differentiating factor is the number of reviews, potential guests may view currently infrequently reviewed apartments as viable booking options as soon as a certain number of reviews is available. Thus, from the perspective of \names{Airbnb}, providing reviews for such apartments is similar to increasing the total number of products that guests consider for booking. \names{Airbnb}'s own referral program points towards the utility of this scenario: users who refer home owners to list their apartment on \names{Airbnb} receive a 75 USD credit, once the newly listed apartment has been booked for the first time. While two scenarios are not equivalent, we assume that for certain apartments the value for \names{Airbnb} of a user switching from a frequently reviewed apartment to an infrequently reviewed apartment is in a similar range.

%%%%%%%%%%%%%%%%%%%%%%%%%%%%%%%%%%%%%%%%%%%%%%%%%%%%%%%%%%%%%%%%%%%%%
%%%%%%%%%%%%%%%%%%%%%%%%%%%%%%%%%%%%%%%%%%%%%%%%%%%%%%%%%%%%%%%%%%%%%
\subsection{Setup}
To answer the questions related to the viability and benefit of our algorithm, we conducted a user study with the following setup. Respondents were asked to consider a scenario in which they were going on a weekend trip for two nights to New York City (U.S.)\footnote{We chose New York City as it has the highest number of \names{Airbnb} listings worldwide.}. Specifically, respondents were asked to consider that they were going alone and considered booking an apartment on a rental site (e.g. \names{Airbnb}). After several introductory questions about the preferences and familiarity with travel accommodations, respondents were given the choice between two apartments. To choose their preferred apartment, respondents were presented several features of each apartment, as shown in Table \ref{table:apartmentinformation}.
\begin{table}[H]
\centering
\begin{tabular}{l l}
 \hline
  Feature & Description \\
 \hline
 Price 				& 		Price per night in USD \\
 Location 			& 		Location on map and distance to Times Square \\
 Picture 			& 		Single picture of the apartment's bedroom \\
 Number of reviews 	& 		Number of reviews from earlier guests \\
 Rating 				& 		One to five star rating \\
 \hline
 \end{tabular}  
\caption[]{Displayed information of each apartment.} 
%\vspace{-2em}
  \label{table:apartmentinformation}
\end{table}

Next to number of reviews and rating, price and location were included because of their importance for guests to decide on travel accommodations \citep{lewis1985predicting}. Further, images have been shown to be important for buyers to evaluate experience goods through online channels \citep{weathers2007effects} and were therefore also included. All five features also correspond to the attributes most commonly mentioned considered for booking hotel rooms through online channels \citep{dickinger2008consumers}.

To obtain the required data about the apartments on \names{Airbnb}, we used the New York City dataset from \names{InsideAirbnb.com}, which is an independent initiative that collects data from \names{Airbnb} for research purpose. The dataset consists of 38,810 apartment listings and includes information about apartment's prices, location, pictures, number of reviews, rating and other features.

%A wide variety of accommodations are offered on \names{Airbnb}, ranging from exclusive penthouse apartments in the city center to ordinary shared bedrooms in the suburb
To make apartments comparable and ensure that they are suited as an accommodation for one person on a weekend trip to New York City, we applied several filters on the list of available apartments, as summarized in Table \ref{table:apartmentfilter}.

\begin{table}[H]
\centering
\begin{tabular}{l l}
 \hline
  Feature $\qquad \qquad \qquad \qquad$ &  Applied filter  \\
 \hline
 Apartment type		& 	Private room				\\ 
 Price per night		& 	80 USD					\\
 Bed type			&	Real bed			  		\\
 Number of beds		& 	1				  		\\
 \hline
 \end{tabular}  
\caption[]{Applied filters on \names{Airbnb} apartment listings.} 
%\vspace{-2em}
  \label{table:apartmentfilter}
\end{table}

In private room apartments, guests have their own room available, but share common areas of the apartment with other people. Private rooms are typically cheaper than entire homes and were selected because of their suitability for solo travelers. The price of 80 USD per night at the lower end of the price range in New York City was selected such that apartments are affordable for a broad range of respondents. Also, apartments were filtered to to have exactly one real bed to ensure the comparability of different apartments.

Of the remaining 700 listings, we grouped the apartment listings based on their location and number of reviews, as shown in Table \ref{table:apartmenttypes}.

\begin{table}[H]
\centering
\begin{tabular}{l l l}
 \hline
  Feature $\qquad \qquad \qquad \qquad$ &  Option 1 & Option 2  \\
 \hline
 Number of reviews	& 	Low ($\leq$ 2) & High ($\geq$ 20)	\\
 Neighborhood		& 	Manhattan & Brooklyn					\\ 

 \hline
 \end{tabular}  
\caption[]{Categories of apartments.} 
%\vspace{-2em}
  \label{table:apartmenttypes}
\end{table}

Combining the two options for number of reviews and neighborhood, we received four different apartment categories. Out of each category, we handpicked five different apartments, ensuring that the bedroom was visible in the picture of every apartment. The location of the 20 apartments in New York City and an example of two presented apartments are provided in Appendix \ref{appendix:userstudy}.

After the respondents decided on their preference between the two randomly selected apartments of the set, they were told that the rental site would like to offer them a special discount for the other apartment, which would reduce the price per night of that apartment. They were then asked to select discount per night that they would like to receive to choose this apartment instead of their initial choice. The options for the answer of this questions were ``0'', ``10'', ``20'', ``30'', ``40'' and ``more than 40''\footnote{We chose these options after testing different increments; responses were consistent for different values.}. Respondents were also instructed to select ''N/A'', if they were not willing to consider the offer and wanted to keep the apartment they had chosen initially. Respondents who selected ``more than 40'' were later asked to provide the exact value they would like to receive. In an open text box, respondents were then asked to specify the factors they considered to decide on the discount they selected.

For the data collecting, the generally preferred option of collecting data directly from \names{Airbnb} was neglected, because of the long lead time that would precede such a cooperation. Instead, we collected user responses from the microtask marketplace \names{Amazon Mechanical Turk}, in which workers receive a compensation for fulfilling small tasks for businesses, developers and researchers. The benefit of using \names{Amazon Mechanical Turk} for research has been demonstrated by \cite{buhrmester2011amazon}. Evaluating the responses on the marketplace, they find that participants are slightly more demographically diverse than are standard internet samples and responses are at least as reliable as those obtained via traditional methods, concluding that \names{Amazon Mechanical Turk} can be used to rapidly obtain high-quality data. To ensure familiarity with New York City, only workers from the United States were considered.

%%%%%%%%%%%%%%%%%%%%%%%%%%%%%%%%%%%%%%%%%%%%%%%%%%%%%%%%%%%%%%%%%%%%%
%%%%%%%%%%%%%%%%%%%%%%%%%%%%%%%%%%%%%%%%%%%%%%%%%%%%%%%%%%%%%%%%%%%%%
\subsection{Apartment Locations}
\begin{figure*}[h!]
\centering
\includegraphics[width=0.5\textwidth]{img/survey/map} \caption{Location of displayed apartments.} \label{figure:map}
\end{figure*}

\subsection{Apartment Choice}

\begin{figure*}[h!]
\centering
\includegraphics[width=0.6\textwidth]{img/survey/screenshot} \caption{Example choice between two apartments.} \label{figure:airbnbsetup}
\end{figure*}

%\clearpage

\subsection{Responses}
%\vspace{-2.5em}
\begin{figure}[H]
  \centering
\subfigure[i: Brooklyn, low; j: Manhattan, high]{\includegraphics{img/survey/Brooklyn-low_Manhattan-high}} \hfill 
\subfigure[i: Brooklyn, high; j: Brooklyn, low]{\includegraphics{img/survey/Brooklyn-high_Brooklyn-low}} \hfill 
\subfigure[i: Brooklyn, low; j: Brooklyn, low]{\includegraphics{img/survey/Brooklyn-low_Brooklyn-low}} \hfill 
\subfigure[i: Manhattan, low; j: Manhattan, high]{\includegraphics{img/survey/Manhattan-low_Manhattan-high}} \hfill 
\subfigure[i: Manhattan, low; j: Manhattan, low]{\includegraphics{img/survey/Manhattan-low_Manhattan-low}} \hfill 
\subfigure[i: Manhattan, high; j: Manhattan, low]{\includegraphics{img/survey/Manhattan-high_Manhattan-low}} \hfill 
\end{figure}

\begin{figure}[H]
\subfigure[i: Manhattan, high; j: Manhattan, high]{\includegraphics{img/survey/Manhattan-high_Manhattan-high}} \hfill 
\subfigure[i: Manhattan, low; j: Brooklyn, high]{\includegraphics{img/survey/Manhattan-low_Brooklyn-high}} \hfill 
\subfigure[i: Manhattan, low; j: Brooklyn, low]{\includegraphics{img/survey/Manhattan-low_Brooklyn-low}} \hfill 
\subfigure[i: Brooklyn, low; j: Manhattan, low]{\includegraphics{img/survey/Brooklyn-low_Manhattan-low}} \hfill 
\subfigure[i: Brooklyn, high; j: Manhattan, high]{\includegraphics{img/survey/Brooklyn-high_Manhattan-high}} \hfill 
\subfigure[i: Brooklyn, low; j: Brooklyn, high]{\includegraphics{img/survey/Brooklyn-low_Brooklyn-high}} \hfill 
\end{figure}

\begin{figure}[H]
\subfigure[i: Brooklyn, high; j: Manhattan, low]{\includegraphics{img/survey/Brooklyn-high_Manhattan-low}} \hfill 
\subfigure[i: Manhattan, high; j: Brooklyn, high]{\includegraphics{img/survey/Manhattan-high_Brooklyn-high}} \hfill 
\subfigure[i: Manhattan, high; j: Brooklyn, low]{\includegraphics{img/survey/Manhattan-high_Brooklyn-low}} \hfill 
\subfigure[i: Brooklyn, high; j: Brooklyn, high]{\includegraphics{img/survey/Brooklyn-high_Brooklyn-high}} \hfill 

\caption{Required discounts for switching from apartment type $i$ to apartment type $j$.}
\end{figure}

%%%%%%%%%%%%%%%%%%%%%%%%%%%%%%%%%%%%%%%%%%%%%%%%%%%%%%%%%%%%%%%%%%%%%
%%%%%%%%%%%%%%%%%%%%%%%%%%%%%%%%%%%%%%%%%%%%%%%%%%%%%%%%%%%%%%%%%%%%%
\subsection{Results: Descriptive Statistics}
The results are separated into two parts. We first provide descriptive statistics about the responses we received and discuss their implications. Next, we test the performance of our \COCP algorith, using the obtained responses about the required discounts. We then discuss the performance of our algorithm in absolute terms and compare it to the independent learning benchmark.

In total, we received 943 responses. Out of all responses, 758 (80.4\%) respondents were willing to accept an offer for their less preferred apartment, given a certain discount per night. The remaining 185 (19.6\%) respondents were not willing to consider the offer and selected ``N/A''. Out of the respondents that were willing to accept the offer, the average required discount for accepting the alternative apartment was 27.9 USD per night. The average required discount for switching from a frequently reviewed apartment to an infrequently reviewed apartment was 29.5 USD per night.  

\begin{figure}[H]
\centering
\includegraphics{img/survey/discounts_sum}

\caption{Total number of responses for different discount options}
\end{figure}

An overview of the results about different pairs of apartments is provided in Table \ref{table:surveyresults}. Detailed results for each combination of apartment types are provided in Appendix \ref{appendix:userstudy}.

\begin{table}[H]
\centering
\begin{tabular}{c c c c c}
 \hline
  Reviews $i$ & Reviews $j$ & Responses & Discount accepted & Avg. required discount\\
 \hline
 High & Low 		&416	&	77.6\%	& 29.5 USD\\
 Low & Low 		&228	&	83.3\% 	& 28.1 USD\\
 High & High 	&219	&	82.2	\%	& 25.4 USD\\
 Low & High 		&80	&	81.3\%	& 25.9 USD\\
 \hline
 \end{tabular}  
\caption[]{Responses for different apartment types.} 
%\vspace{-2em}
  \label{table:surveyresults}
\end{table}

As can be inferred from Table \ref{table:surveyresults}, 496 respondents were given a choice between a frequently and an infrequently reviewed apartment. Out of these respondents 83.9\% respondents chose the frequently reviewed apartment, while only 16.1\% respondents chose the infrequently reviewed apartment. Also, the average required discount per night was 3.5 USD higher when the alternative choice was an infrequently reviewed apartment.

In the responses to the open question about the factors respondents considered to decide on the discount, we captured the frequency at which different factors were mentioned by defining several keywords for each factor, as listed in Table \ref{table:survekeywords}. The frequency at which each factor was mentioned is shown in Figure \ref{figure:surveywords}.

\begin{table}[H]
\centering
\begin{tabular}{l l}
 \hline
  Factor & Keywords\\
 \hline
 Location 				& 		location, neighborhood, distance, close, away, transport, commute,  \vspace{-0.2em}\\ 
 						& 		brooklyn, manhattan, times square\\
 Reviews 				& 		reviews, rating, star \\
 Price 					& 		price, expensive, cheap \\
 Picture					& 		picture, image, photo, look \\
 \hline
 \end{tabular}  
\caption[]{Keywords for each factor.} 
  \label{table:survekeywords}
\end{table}

\begin{figure}[H]
\centering
\includegraphics{img/survey/text_mentions}

\caption{Mentioned factors for deciding on the required discount.} \label{figure:surveywords}
\end{figure}

The most frequently mentioned factor was location with 477 mentions (50.6\% of responses). Next, factors related to customer reviews were mentioned 309 times (32.8\% of all responses). Factors related to prices were mentioned 182 times (19.3\% of all responses) and factors related to the picture 169 times (17.9\% of all responses). Also, 12 respondents mentioned concerns regarding trust towards infrequently reviewed apartments, out of which 8 were not willing to consider an alternative apartment. 

%%%%%%%%%%%%%%%%%%%%%%%%%%%%%%%%%%%%%%%%%%%%%%%%%%%%%%%%%%%%%%%%%%%%%
%%%%%%%%%%%%%%%%%%%%%%%%%%%%%%%%%%%%%%%%%%%%%%%%%%%%%%%%%%%%%%%%%%%%%
